# Supplementary material for: Goal Space Abstraction in Hierarchical Reinforcement Learning via Set-Based Reachability Analysis
Source: arXiv:2309.07675 source file (2023-11-22)
Supplement: Supplementary file 1 [file appendix.tex]

\appendix
\section*{The k-Forward Model}
The $k-$forward model $\fwdmodel: \states \times \partitions \rightarrow \states $ is trained to predict the state $s'$ reached after applying $\lowpolicy{s}{\partition'}$ for $k$ steps.
In practice, we use a fully connected neural network to approximate this relation. This network is composed of two layers with 16 neurons each. We use an MSE loss function to train the network with a learning rate of $0.1$.

The forward model $F_k(s,G)$ approximates the state reached when applying a policy $\lowpolicy{s}{G}$ for $k$ steps. Since this policy is changing during training. The model $F_k$ is regularly updated. This can be considered as a similar process to off-policy DRL approaches where the policy networks keep track of the trained policy's generated rewards. Importantly, the reachability of a policy is only analysed after the policy has stabilised. We rely on $F_k$'s errors to determine this criteria. More precisely, we assume that if the corresponding forward model's error remains stable across multiple episodes, and since it is trained on data generated by $\pi_{\text{Low}}$, then the low-level policy is stable.

\section*{Discussing non-stationarity in \acronym}
Non-stationarity issues, common in HRL algorithms, refer to a high-agent's experience replay containing data that stems from changing behaviours. As the low-level policies are trained, their outcome changes leading to replay data not reflecting the behaviour of the current agents. Non-stationarity is avoided in \acronym due to the advantages offered by its structure. First, \acronym's high-level agent relies on Q-learning for training $\highpolicy$ and does not need to rely on a replay buffer. This naturally lessens the dependence on old experiences and introduces less errors in training. Second, the refinement mechanism is activated once low-level policies have stabilised meaning that non-stationarity will not affect the following high-level training.

\section*{The Maze environment}
In the maze environment, the actions affect the acceleration of the agent and consequently its velocities and positions. Each action either increases or decreases the acceleration value by an increment of $0.1$ at a timestep.
UP/DOWN affect the vertical acceleration $a_y(t)$ while the RIGHT and LEFT action change the horizontal acceleration $a_x(t)$. When picking an action across an a certain axis, the acceleration value of the unpicked axis moves closer to 0.
Concretely, these actions affect the corresponding velocities as $v_x(t) = max( min(v_x(t-1) + a_x(t),1), -1)$ and $v_y(t+1) = max(min(v_y(t-1) + a_y(t), 1), -1)$.

\section*{Hyperparameters}
We tuned the DQN networks by testing the low-level policy convergence in small, unobstructed rooms. This allows us to simulate the required behaviour from low-level policies. The Q-network for all approaches is thus composed of 2 hidden layers (with 16 and 32 neurons respectively). The learning rate is set to $0.01$. The low-level agent uses an $\epsilon$-greedy policy with $\epsilon$ annealed exponentially by a factor of 0.9995 from $\epsilon_{initial}=1$ to $\epsilon_{min}=0.01$. The target networks are updated every 20 time steps.
For Feudal HRL with concrete representations, both Actor and Critic networks of DDPG have 2 hidden layers with 16 and 32 neurons respectively. Feudal HRL with LSTM adds to that an LSTM layer with 32 units. 

For every approach, a new goal is sampled by the high-level each $k=5$ steps. $k$ is chosen intuitively as being the mean number of steps an agent could take to exit a room in our environment. The maximal number of steps per episode is set to $200$.

\section*{Additional Results}
We conducted additional experiments on other maze configurations to assess our results under other types of environment variations. 
\noindent
First, we switch the start and exit positions in the U-shaped Maze. This is a form of task modification where the environment is unchanged. Fig.\ref{fig:U-shaped_Switch} shows that the transferred version of \acronym~ starts learning faster than the from-scratch version. They achieve comparable behaviours in the later stages of learning. This is explained by the fact that \acronym~-Transfer can train its low-level policies faster with the provided precise representation whereas the from-scratch version has to first identify the subgoal representation before it can train efficient low-level policies. It is to note that \acronym~-Transfer in this task does not refine the goal space as the transferred partition already satisfies the reachability property.

\begin{figure}[tbh]
    \centering
    \includegraphics[width=1.0\columnwidth]{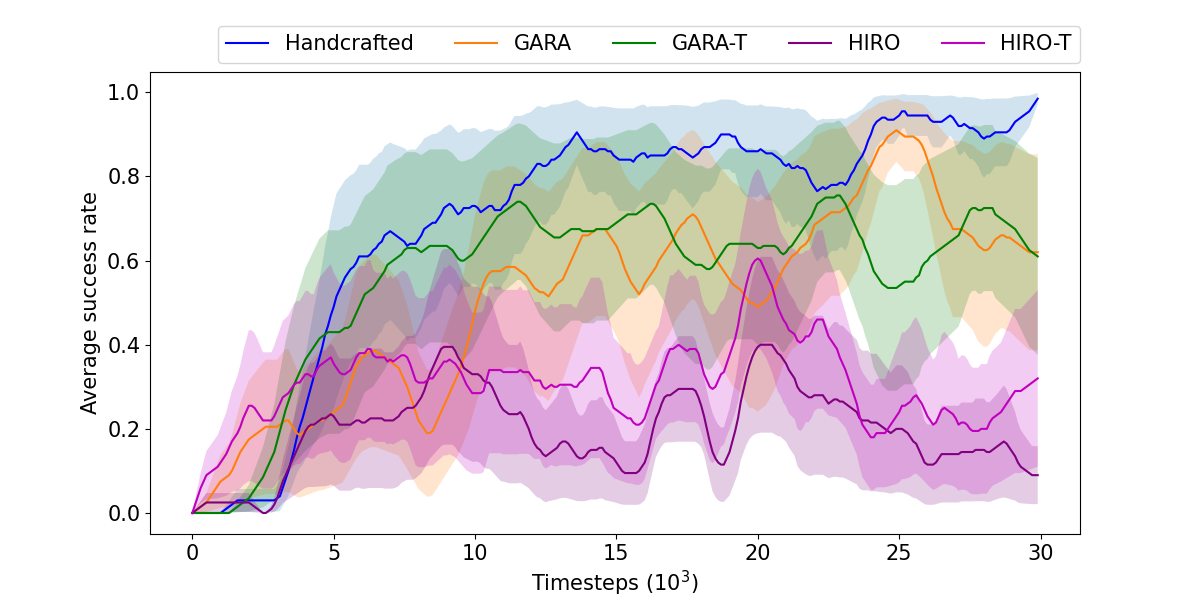}
    \caption{Evaluation on U-shaped Maze with switched Start/Exit}
    \label{fig:U-shaped_Switch}
\end{figure}

\noindent
Second, we expand the size of the environment and propose an N-shaped maze Fig.\ref{fig:nshapedMaze}. This is a configuration designed to assess transfer performance in a larger environment.
\begin{figure}[tbh]
    \centering
    \includegraphics[width=0.4\columnwidth]{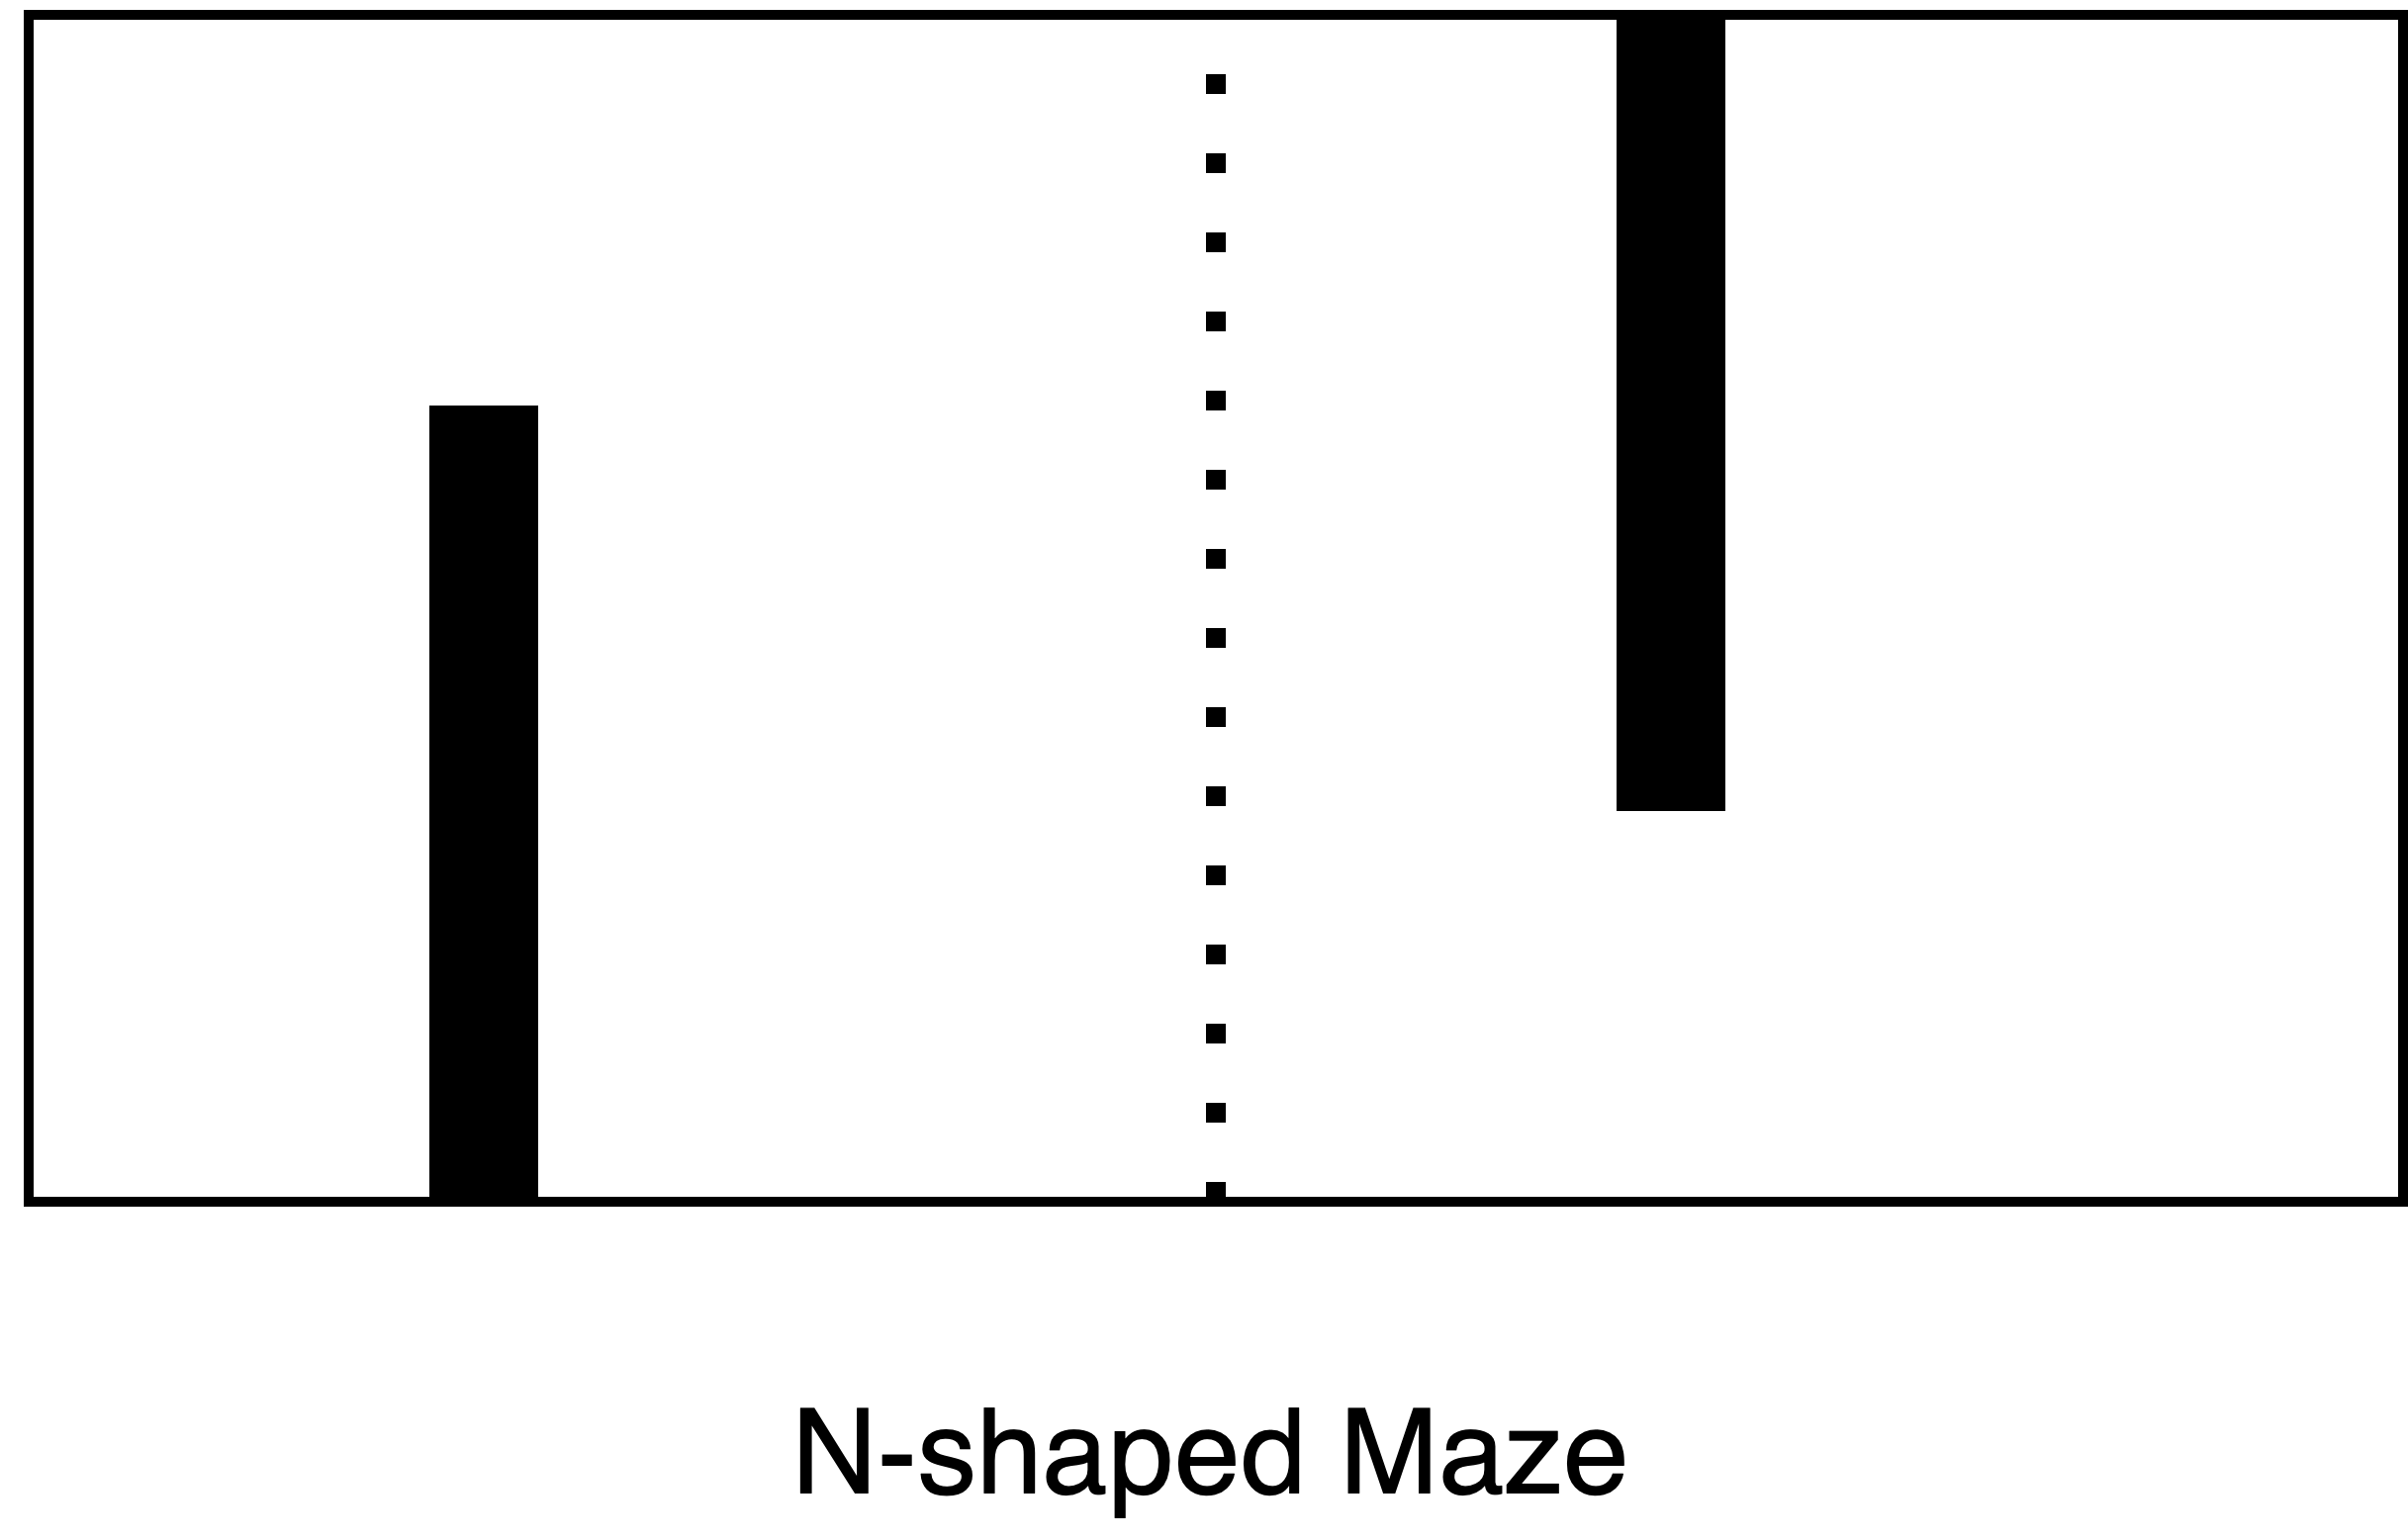}
    \caption{N-shaped Maze}
    \label{fig:nshapedMaze}
\end{figure}
Fig.\ref{fig:N-Maze} shows that the transferred version of \acronym~ benefits greatly from the transferred representation. It manages to learn faster and better performing policies even compared to the Handcrafted approach. This is due to the handcrafted approach that, while intuitive, does not sufficiently decompose the task and adapt it to the capabilities of the low-level agent Fig.\ref{fig:N-Maze_handcrafted_repr}. This is especially more prominent in the middle section of the maze. On the other hand, \acronym~is able to address the ambiguity of the large middle section as seen in Fig.\ref{fig:N-Maze_repr1}, Fig.\ref{fig:N-Maze_repr2} and Fig.\ref{fig:N-Maze_repr3}.
\begin{figure}[H]
    \centering
    \includegraphics[width=1.0\columnwidth]{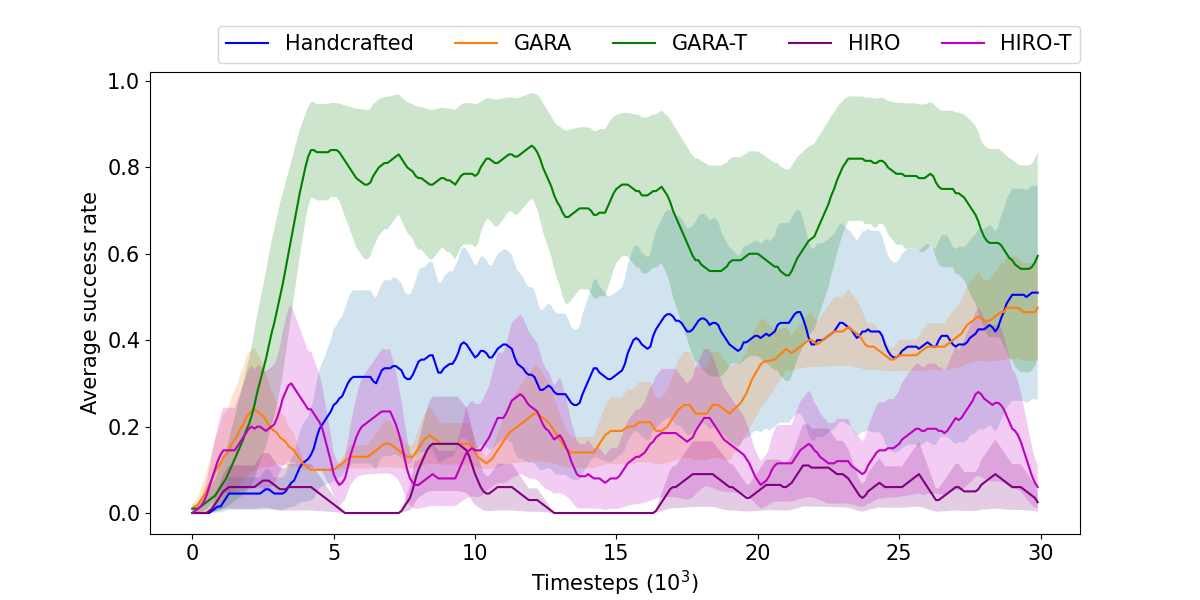}
    \caption{Evaluation on N-shaped Maze}
    \label{fig:N-Maze}
\end{figure}

\begin{figure}[tbh]
    \centering
    \subfloat[Handcrafted representation \label{fig:N-Maze_handcrafted_repr}]{\includegraphics[width=0.22\columnwidth]{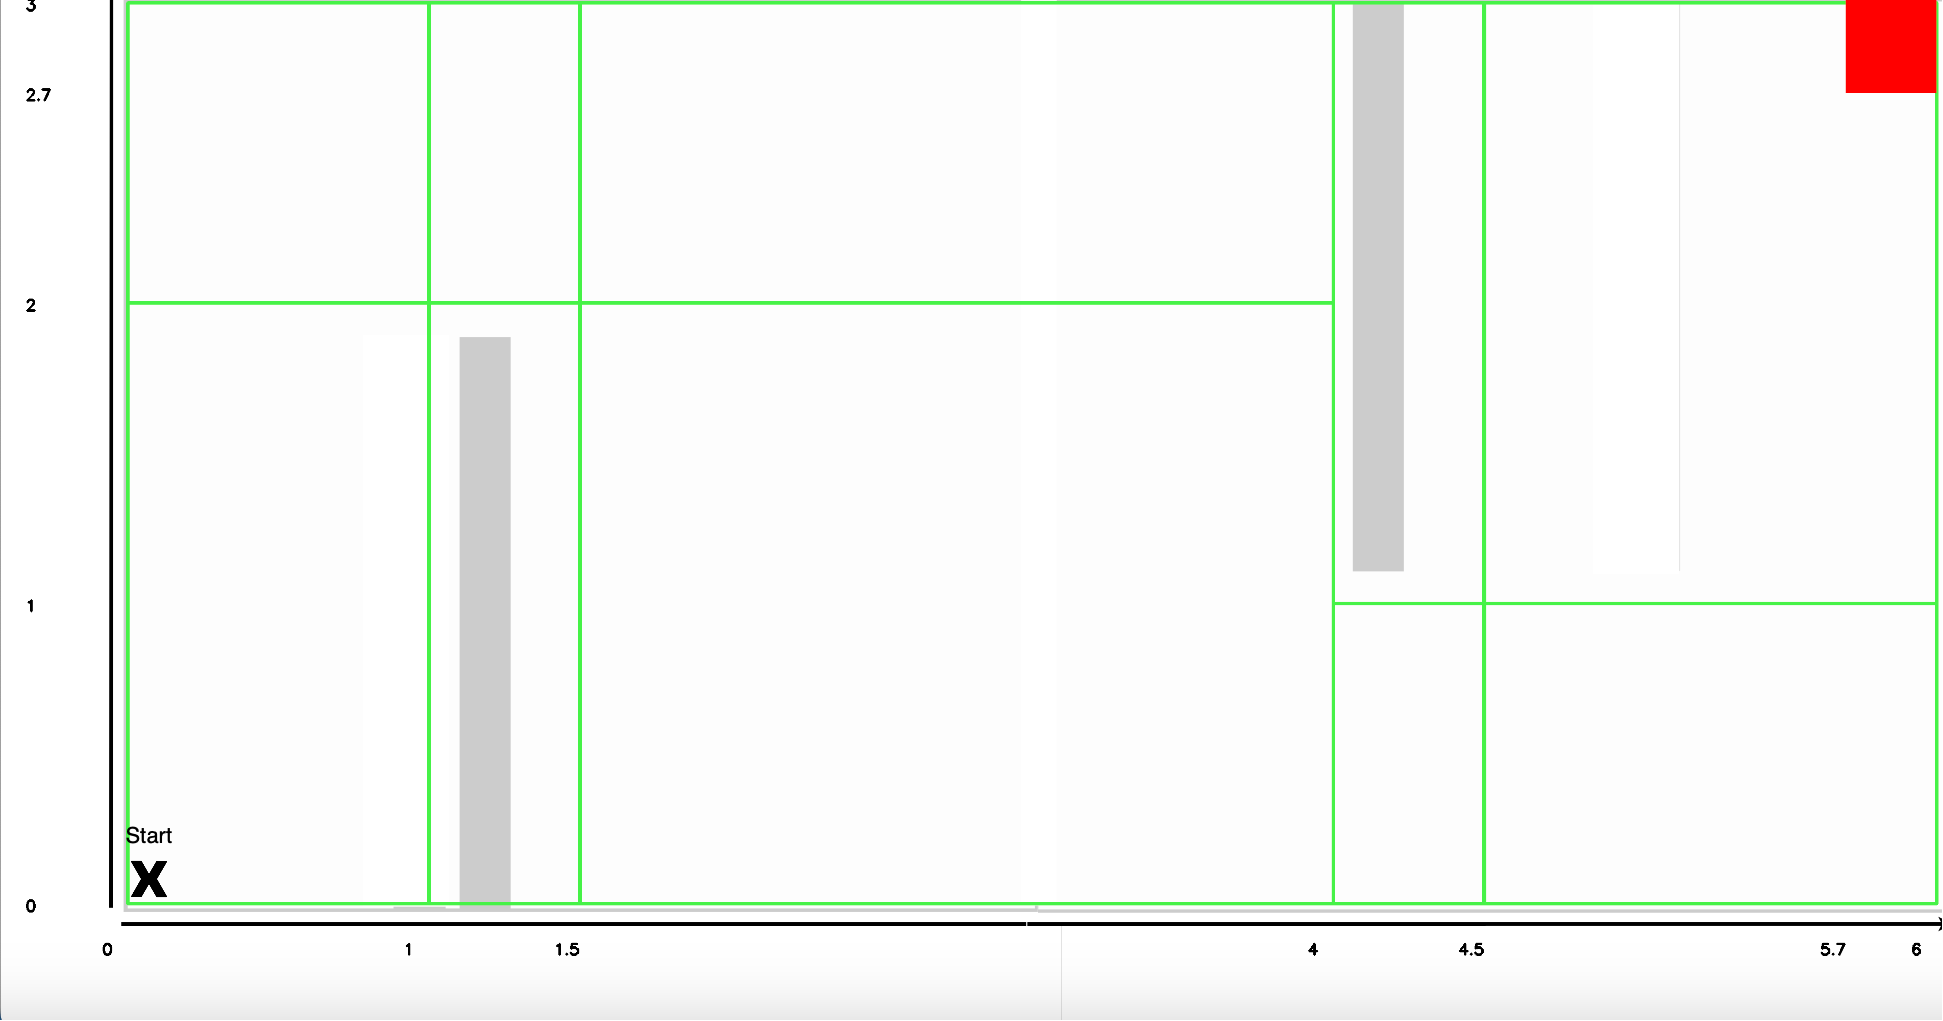}} 
    \hfill
    \subfloat[Transferred $\partitions$ for \acronym-Transfer \label{fig:N-Maze_repr1}]{\includegraphics[width=0.22\columnwidth]{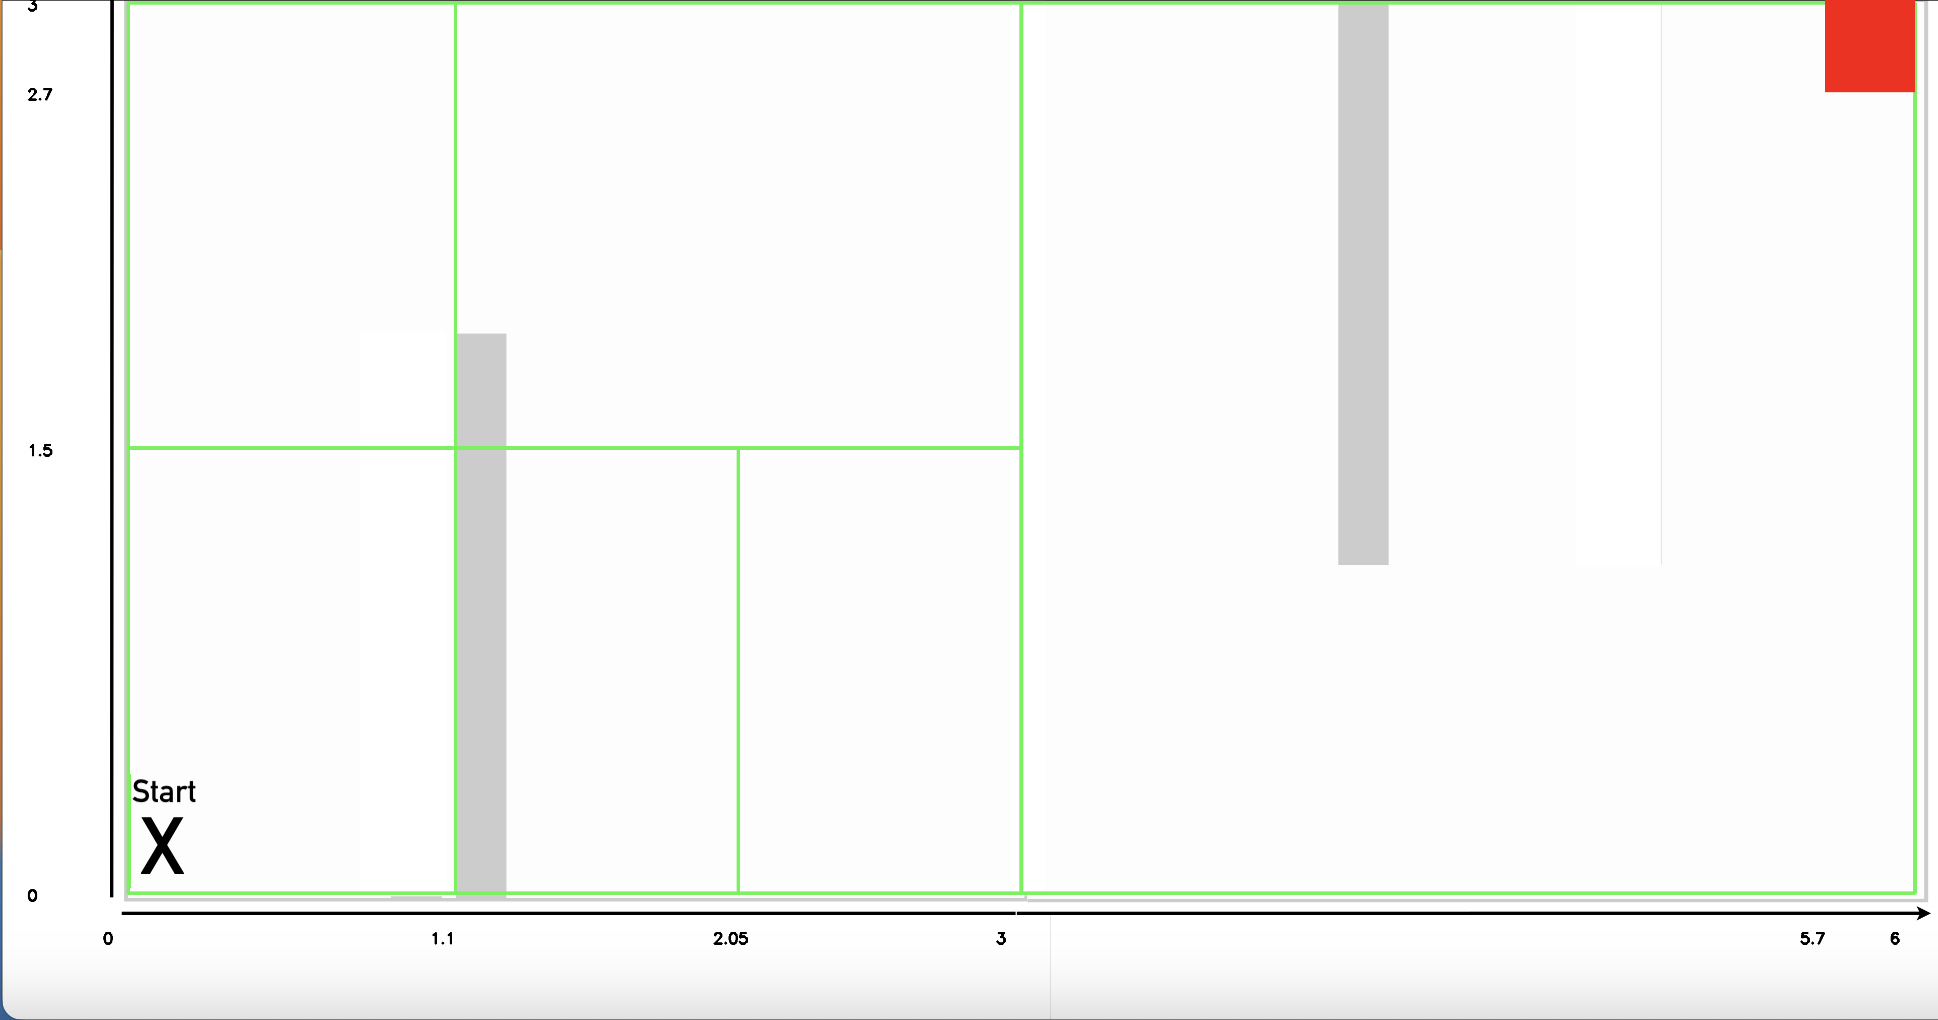}}
    \hfill
    \subfloat[$\partitions$ learned by \acronym~-Transfer after $10^3$ steps \label{fig:N-Maze_repr2}]{\includegraphics[width=0.22\columnwidth]{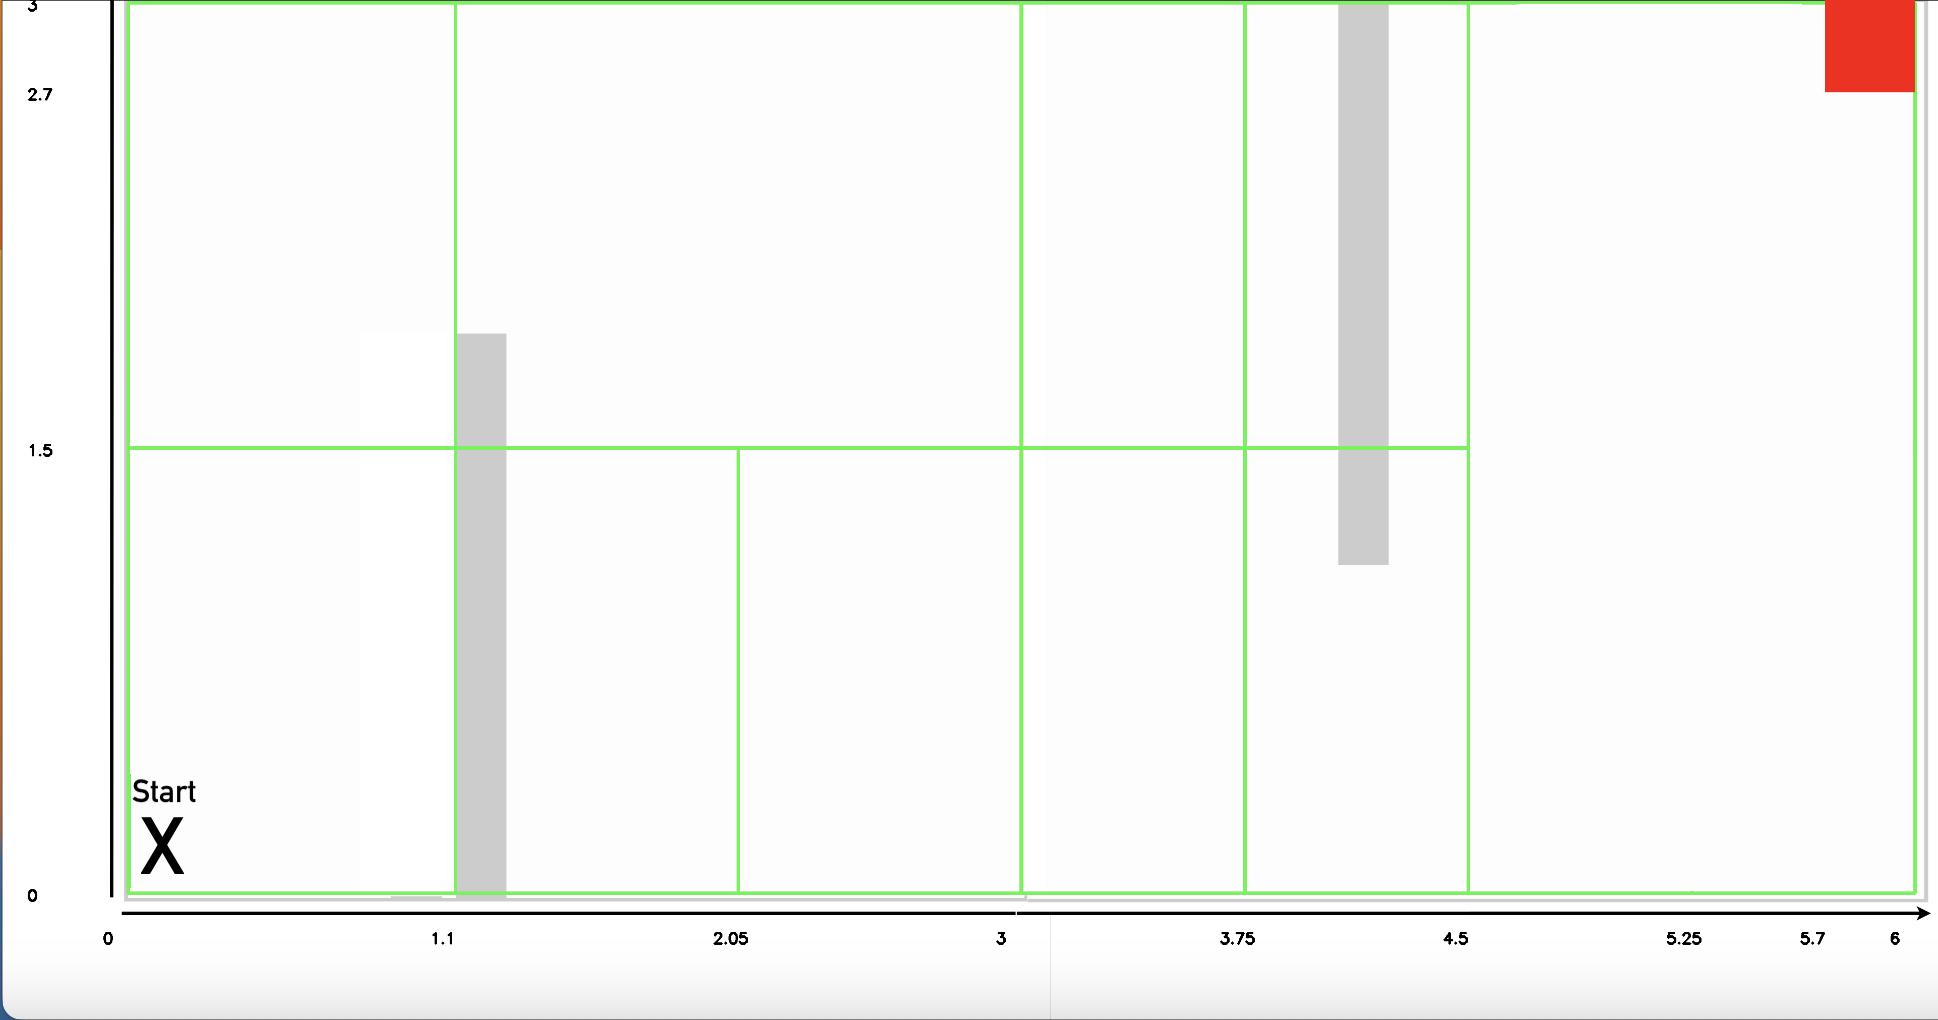}} 
    \hfill
    \subfloat[Final $\partitions$ learned by \acronym~-Transfer \label{fig:N-Maze_repr3}]{\includegraphics[width=0.22\columnwidth]{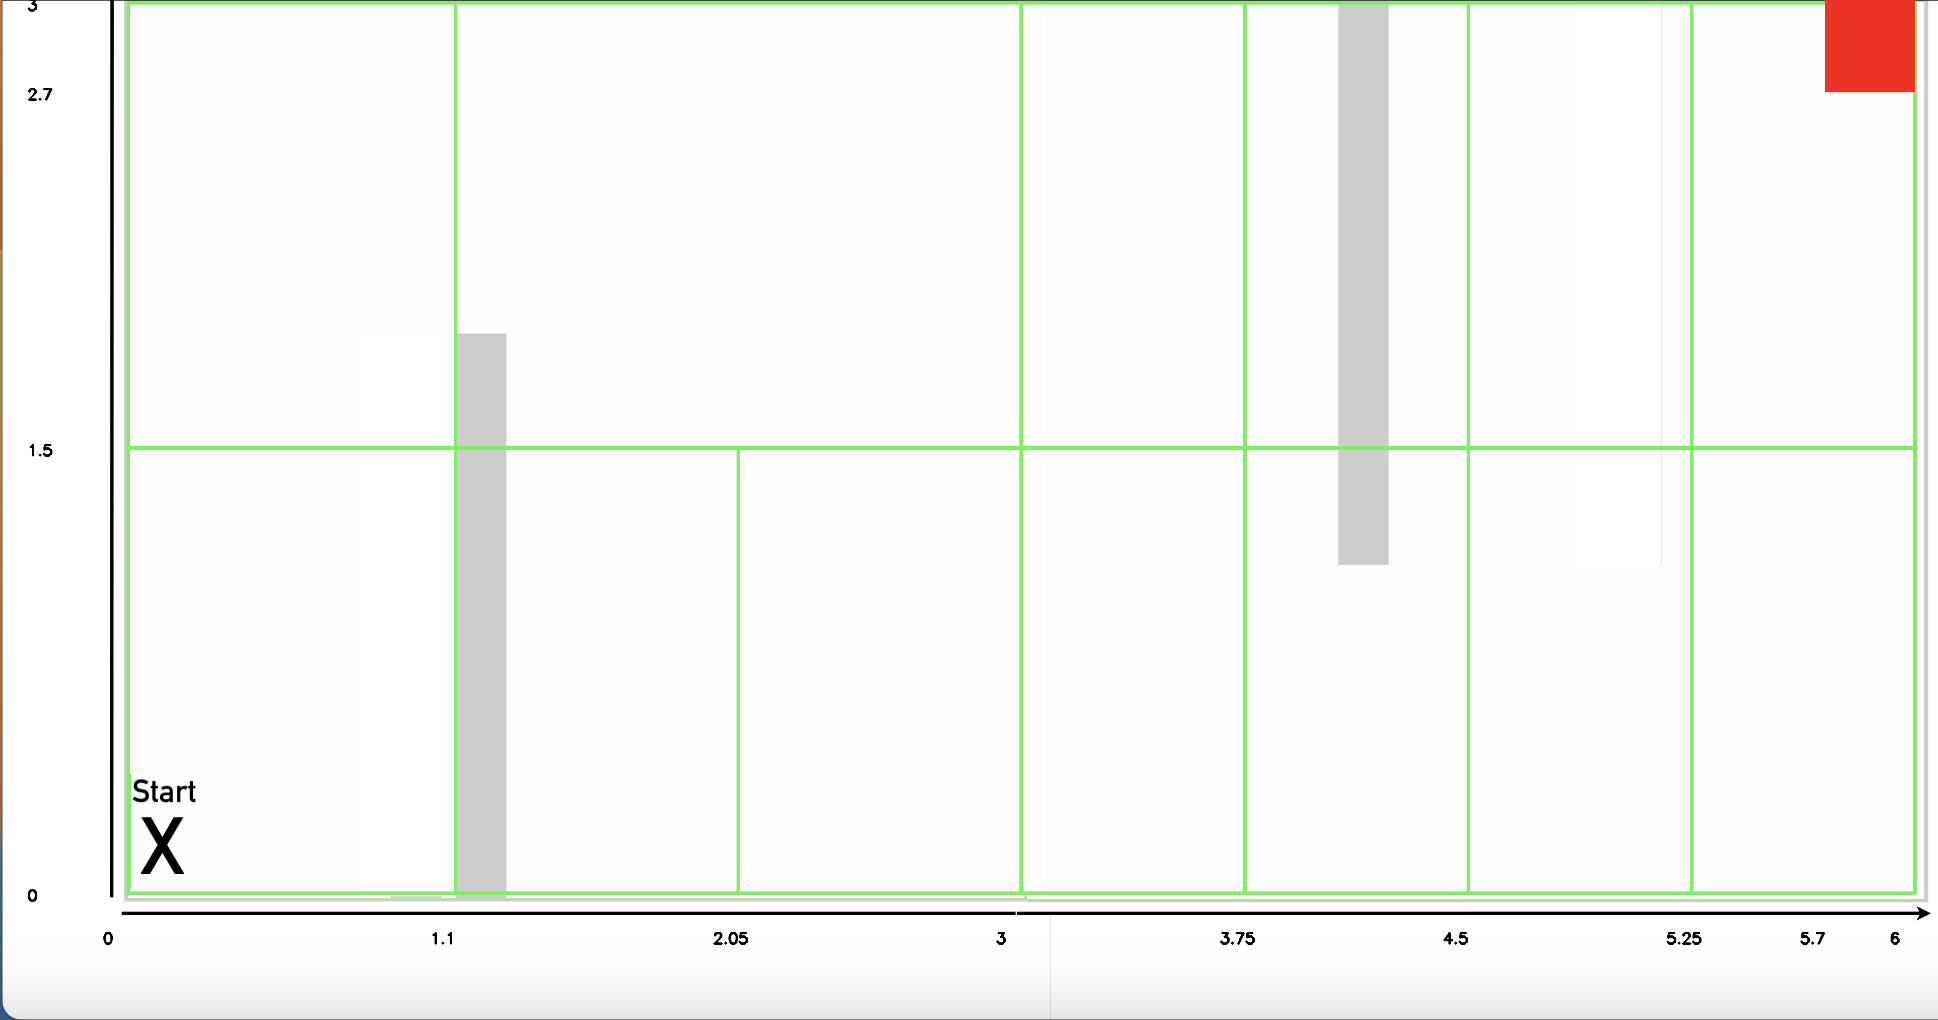}} 
     \caption{Representation of the subgoal space in the N-Maze configuration}
    \label{fig:N-Maze_repr}
\end{figure}
